# Supplementary material for: Concentration banding instability of a sheared bacterial suspension
Source: arXiv:1808.07805 ancillary file (2018-08-23)
Supplement: Supplementary file 1 [file Supplementary_Information_modified.pdf]

# Supplementary Information

## I. NUMERICAL SOLUTION OF $\Omega_0(\mathbf{p})$

The governing equation for the probability density of bacterium position and orientation, with the bacteria undergoing a combination of a run-and-tumble motion and rotary diffusion at the micro-scale (where the tumbles assumed to be perfectly random) is given by [S10, S11]:

$$\frac{\partial \Omega}{\partial t} + U_b \mathbf{p}.\nabla_{\mathbf{x}}\Omega - D_r \nabla_p^2 \Omega + \nabla_p \cdot (\dot{\mathbf{p}}\Omega) + \frac{1}{\tau}[\Omega - \int d\mathbf{p}^{'} \frac{1}{4\pi}\Omega(\mathbf{p}^{'})] = 0. \tag{S1}$$

The equations of continuity and motion for the bacterial suspension are given by:

$$\begin{aligned} \mu \nabla^2 \mathbf{u} &= -\nabla \cdot \Sigma^B, \\ \nabla \cdot \mathbf{u} &= 0. \end{aligned} \tag{S2}$$

Here, $\Sigma^B = -\mu \mathcal{C} n_0 L^2 U_b \int d\mathbf{p}\Omega(\mathbf{p})(\mathbf{pp} - I/3)$ is the active stress due to the bacterium force dipole [S2, S11], where $\mu, \mathcal{C}, n_0, L$ denote the fluid viscosity, bacterial force dipole strength, bacterial number density and bacterium length respectively. In the general case, $\Sigma^B$ has an additional passive stress contribution arising from the bacterium inextensibility. At low $Pe$, the regime of interest in this work, the primary physical affect of the passive stress is to lead to an enhanced viscosity. Since its affect, at $Pe = 0$, has been examined before, here we neglect it to focus on the active-stress and concentration coupling [S11].

The kinetic equation (Eq. S1) and equations of motion and continuity (Eq. S2) are non-dimensionalized by using $\tau$, $H$, $U_\infty$ and $\mu\tau^{-1}$ as the scales for time, length, velocity, stress and the resulting non-dimensional equations are

$$\frac{\partial \Omega}{\partial t} + \epsilon \mathbf{p}.\nabla_{\mathbf{x}}\Omega - D_r \tau \nabla_p^2 \Omega + Pe \nabla_p \cdot (\dot{\mathbf{p}}\Omega) + [\Omega - \int d\mathbf{p}^{'} \frac{1}{4\pi}\Omega(\mathbf{p}^{'})] = 0, \tag{S3}$$

and

$$Pe \frac{\partial^2 u}{\partial z^2} = \mathcal{A} \frac{\partial}{\partial z} \int d\mathbf{p}\Omega(z, \mathbf{p}) p_1 p_3. \tag{S4}$$

Here, $\mathbf{u} = \mathbf{\Gamma} \cdot \mathbf{x}$ is the base state shear velocity field, and for the simple shear flow considered here $\mathbf{\Gamma} = \dot{\gamma} 1_x 1_z$. The non-dimensional parameters that appear in the system of equations above are the bacterial Knudsen number, $\epsilon = U_b \tau / H$, the Peclet number $Pe = U_\infty \tau / H$ which measures the relative importance of flow and intrinsic reorientation time scales, and the activity number $\mathcal{A} = C n_0 L^2 U_b \tau$ which is a dimensionless measure of the active dipole density. The bacterium orientation, in the spherical coordinate system chosen for the subsequent analysis, is

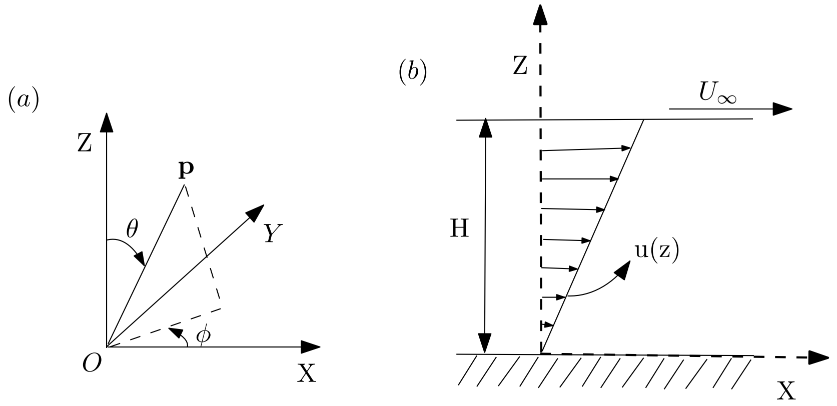


FIG. S1: Schematic showing the (a) coordinate system of a bacterium (b) bacterial suspension subjected to simple shear

depicted in Fig. S1.

In order to examine the linear stability of the bacterial suspension subjected to a simple shear, we consider a small perturbation, with an amplitude $A \ll 1$, of the homogeneously sheared base state:

$$u(z,t) = u_0(z) + Au_1(z,t) + \cdots . \tag{S5}$$

Correspondingly, the bacterial probability density is expressed as:

$$\Omega(\mathbf{p}, z, t) = \Omega_0(\mathbf{p}) + A\Omega_1(z, \mathbf{p}, t) + \cdots . \tag{S6}$$

Substituting Eq. S5 and S6 into S3, one has the following equations at successive orders:

$$\mathcal{O}(1) : Pe\nabla_p \cdot (\dot{\mathbf{p}}^{'}\Omega_0) + [\Omega_0 - \int d\mathbf{p}^{'} \frac{1}{4\pi}\Omega_0(\mathbf{p}^{'})] - D_r\tau\nabla_p^2\Omega_0 = 0, \tag{S7}$$

and

$$\mathcal{O}(A) : \frac{\partial\Omega_1}{\partial t} + \epsilon\mathbf{p}.\nabla_{\mathbf{x}}\Omega_1 - D_r\tau\nabla_p^2\Omega_1 + Pe\nabla_p \cdot (\dot{\mathbf{p}}^{'}\Omega_1) + Pe\dot{\gamma}_1\nabla_p \cdot (\dot{\mathbf{p}}^{'}\Omega_0) + [\Omega_1 - \int d\mathbf{p}^{'} \frac{1}{4\pi}\Omega_1(\mathbf{p}^{'})] = 0. \tag{S8}$$

Here, $\dot{\mathbf{p}}^{'} = \mathbf{E}^{'}.\mathbf{p} + \omega^{'}.\mathbf{p} - \mathbf{p}(\mathbf{E}^{'} : \mathbf{pp})$ with $\mathbf{E}^{'} = \frac{1}{2}(\delta_{i1}\delta_{j3} + \delta_{i3}\delta_{j1})$, $\omega^{'} = \frac{1}{2}(\delta_{i1}\delta_{j3} - \delta_{i3}\delta_{j1})$, $\dot{\gamma}_1 = \frac{\partial u_1}{\partial z}$ is the perturbation simple shear flow (the topology of the perturbation flow remains identical to the base-sate, on account of the assumption of layering perturbations) and $\delta_{ij}$ is the Kronecker delta. Equation S7 describes the homogeneous anisotropic base-state, while Eq. S8 describes the dynamics at linear order in the perturbation amplitude.

## II. THE BASE STATE

In the following, we describe the numerical scheme for the calculation of base-state probability density ($\Omega_0$) and the base-state stress $\Sigma_0$.

### A. Numerical solution of the base-state probability density

Considering $\nabla_p \cdot (\dot{\mathbf{p}}^{'}\Omega_0)$, the first term in Eq. S7, substituting $\dot{\mathbf{p}}^{'}$, and after simplification, one may write:

$$\begin{aligned} \nabla_p.(\dot{\mathbf{p}}^{'}\Omega_0(\mathbf{p})) &= \cos^2\theta\cos\phi\frac{\partial\Omega_0}{\partial\theta} - \cot\theta\sin\phi\frac{\partial\Omega_0}{\partial\phi} - 3\Omega_0\sin\theta\cos\theta\cos\phi \\ &= i\cos^2\theta\mathcal{L}_y(\Omega_0) - i\sin\theta\cos\theta\sin\phi\mathcal{L}_z(\Omega_0) - 3\sin\theta\cos\theta\cos\phi\Omega_0, \end{aligned} \tag{S9}$$

where the operators

$$\begin{aligned} \mathcal{L}_y &= -i\cos\phi\frac{\partial}{\partial\theta} + i\cot\theta\sin\phi\frac{\partial}{\partial\phi}, \\ \mathcal{L}_z &= -i\frac{\partial}{\partial\phi}. \end{aligned}$$

Now, rewriting Eq. S9 with the coefficients of partial derivatives written in terms of spherical harmonics:

$$\begin{aligned} \nabla_p.(\dot{\mathbf{p}}^{'}\Omega_0(\mathbf{p})) &= \left(\frac{2}{3}\sqrt{\frac{4\pi}{5}}Y_2^0 + \frac{1}{3}\sqrt{4\pi}Y_0^0\right) i\mathcal{L}_y(\Omega_0) + \sqrt{\frac{2\pi}{15}}\left(Y_2^{-1} + Y_2^1\right)\mathcal{L}_Z(\Omega_0) \\ &- 3\sqrt{\frac{2\pi}{15}}\left(Y_2^{-1} - Y_2^1\right)\Omega_0. \end{aligned} \tag{S10}$$

Further expanding the orientation probability density as:

$$\Omega_0(\mathbf{p}) = \sum_{l=0}^{\infty}\sum_{m=-l}^{l} a_{l,m} Y_l^m(\mathbf{p}) \tag{S11}$$

with $a_{l,m}$ being the unknown series coefficients, and substituting in the above equation leads to:

$$\begin{aligned}\nabla_p.(\dot{\mathbf{p}'}\Omega_0(\mathbf{p})) &= \sum_{l=0}^{\infty}\sum_{m=-l}^{l} a_{l,m}\left[\left(\frac{2}{3}\sqrt{\frac{4\pi}{5}}Y_2^0 + \frac{1}{3}\sqrt{4\pi}Y_0^0\right) i\mathcal{L}_y \mid Y_l^m >\right. \\ &+ \left.\sqrt{\frac{2\pi}{15}}\left(Y_2^{-1}+Y_2^1\right)\mathcal{L}_Z \mid Y_l^m > -3\sqrt{\frac{2\pi}{15}}\left(Y_2^{-1}-Y_2^1\right)Y_l^m\right],\end{aligned} \tag{S12}$$

where $\mathcal{L}_i \mid Y_l^m >= \mathcal{L}_i(Y_l^m)$.

Using Eq. S11, S12 and the following results [S1, S8]

$$\begin{aligned} i\mathcal{L}_y \mid Y_l^m > &= \frac{1}{2}\left[\sqrt{l(l+1)-m(m+1)}Y_l^{m+1} - \sqrt{l(l+1)-m(m-1)}Y_l^{m-1}\right], \\ \mathcal{L}_z \mid Y_l^m > &= mY_l^m \end{aligned} \tag{S13}$$

in Eq. S7, we have

$$\begin{aligned}&\sum_{l=0}^{\infty}\sum_{m=-l}^{l} a_{l,m}\left\{\left[Y_l^m - \int d\mathbf{p}'\frac{1}{4\pi}Y_l^m(\mathbf{p}')\right] - D_r\tau\nabla_p^2 Y_l^m + Pe\left[\sqrt{\frac{2\pi}{15}}\left(Y_2^{-1}+Y_2^1\right)mY_l^m\right.\right. \\ &+\left(\frac{1}{3}\sqrt{\frac{4\pi}{5}}Y_2^0 + \frac{1}{6}\sqrt{4\pi}Y_0^0\right)\left[\sqrt{l(l+1)-m(m+1)}Y_l^{m+1} - \sqrt{l(l+1)-m(m-1)}Y_l^{m-1}\right] \\ &\left.\left.-3\sqrt{\frac{2\pi}{15}}\left(Y_2^{-1}-Y_2^1\right)Y_l^m\right]\right\} = 0.\end{aligned} \tag{S14}$$

Multiplying the above equation with a conjugate spherical harmonic $Y_r^{s^*}(\mathbf{p})$, and using the orthogonality of the spherical harmonics on the unit sphere, gives the following system of linear equations for the $a_{l,m}$'s:

$$\begin{aligned}&\sum_{l=0}^{\infty}\sum_{m=-l}^{l} a_{l,m}\left\{\left[1+D_r\tau l(l+1)\right]\delta_{lr}\delta_{ms} - \delta_{l0}\delta_{m0}\delta_{r0}\delta_{s0} + Pe\left[m\sqrt{\frac{2\pi}{15}}\left(< r,s|Y_2^{-1}|l,m> + < r,s|Y_2^1|l,m>\right)\right.\right. \\ &+\sqrt{l(l+1)-m(m+1)}\left(\frac{1}{3}\sqrt{\frac{4\pi}{5}} < r,s|Y_2^0|l,m+1> + \frac{\sqrt{4\pi}}{6} < r,s|Y_0^0|l,m+1>\right) \\ &-\sqrt{l(l+1)-m(m-1)}\left(\frac{1}{3}\sqrt{\frac{4\pi}{5}} < r,s|Y_2^0|l,m-1> + \frac{\sqrt{4\pi}}{6} < r,s|Y_0^0|l,m-1>\right) \\ &\left.\left.-3\sqrt{\frac{2\pi}{15}}\left(< r,s|Y_2^{-1}|l,m> - < r,s|Y_2^1|l,m>\right)\right]\right\} = 0.\end{aligned} \tag{S15}$$

In the above equation

$$\begin{aligned} < a,b|Y_l^m|p,q> &= \int d\mathbf{p}Y_a^{b^*}(\mathbf{p})Y_l^m(\mathbf{p})Y_p^q(\mathbf{p}) \\ &= (-1)^b\sqrt{\frac{(2a+1)(2l+1)(2p+1)}{4\pi}}\begin{pmatrix} a & l & p \\ 0 & 0 & 0\end{pmatrix}\begin{pmatrix} a & l & p \\ -b & m & q\end{pmatrix},\end{aligned} \tag{S16}$$

where the Wigner-3j symbols, $\begin{pmatrix} l1 & l2 & l3 \\ m1 & m2 & m3\end{pmatrix}$ will be evaluated by using the Racah formula[S1, S5, S8].

Imposing the normalization condition on the total probability density, with $n_1(z)$ below being the perturbation number density, one obtains:

$$\int d\mathbf{p}\Omega(\mathbf{p},z,t) = \int d\mathbf{p}(\Omega_0 + A\Omega_1(\mathbf{p},z,t) + \cdots) = 1 + An_1(z,t) + \cdots\,, \tag{S17}$$

which implies

$$\int \Omega_0(\mathbf{p})d\mathbf{p} = 1. \tag{S18}$$

Substituting Eq. S11 in the above equation, one would get

$$a_{0,0} = 1/\sqrt{4\pi}. \tag{S19}$$

Using $a_{0,0}$ from Eq. S19, in Eq. S15 gives

$$\begin{aligned}
&\sum_{l=1}^{\infty}\sum_{m=-l}^{l} a_{l,m}\Bigg\{[1+D_r\tau l(l+1)]\,\delta_{lr}\delta_{ms} + Pe\Bigg[m\sqrt{\frac{2\pi}{15}}\left(<r,s|Y_2^{-1}|l,m> + <r,s|Y_2^{1}|l,m>\right)\\
&+\sqrt{l(l+1)-m(m+1)}\left(\frac{1}{3}\sqrt{\frac{4\pi}{5}}<r,s|Y_2^{0}|l,m+1> + \frac{\sqrt{4\pi}}{6}<r,s|Y_0^{0}|l,m+1>\right)\\
&-\sqrt{l(l+1)-m(m-1)}\left(\frac{1}{3}\sqrt{\frac{4\pi}{5}}<r,s|Y_2^{0}|l,m-1> + \frac{\sqrt{4\pi}}{6}<r,s|Y_0^{0}|l,m-1>\right)\\
&-3\sqrt{\frac{2\pi}{15}}\left(<r,s|Y_2^{-1}|l,m> - <r,s|Y_2^{1}|l,m>\right)\Bigg]\Bigg\} = Pe\sqrt{\frac{3}{10}}\left(<r,s|Y_2^{-1}|0,0> - <r,s|Y_2^{1}|0,0>\right),
\end{aligned} \tag{S20}$$

which may now be solved for the $a_{l,m}$'s with $(l,m) \neq (0,0)$. We truncate the series in Eq. S20 for a finite number of unknown coefficients $a_{l,m}$, that is truncate $l$ at $L_{max}$ and then solve the resulting system of linear equations numerically. The convergence of the results is checked with respect to the number of harmonics retained throughout the work. We find that at larger $Pe$, greater number of harmonics are required for convergence. For the results presented in the main paper, $L_{max} = 10$ was found to be sufficient.

### B. Base state stress

Substituting Eq. S5, S6 in Eq. S4, then one may write the base state stress as:

$$\Sigma_0 = Pe\frac{\partial u_0}{\partial z} - \mathcal{A}\int d\mathbf{p}\Omega_0(\mathbf{p})p_1p_3. \tag{S21}$$

Using $u_0(z) = z$ and $\Omega_0(\mathbf{p})$ expansion (from Eq. S11) in the above equation and employing the orthogonal properties of spherical harmonics, we get

$$\Sigma_0 = Pe - \mathcal{A}\sqrt{\frac{2\pi}{15}}\left(a_{2,-1} - a_{2,1}\right). \tag{S22}$$

The base-state being homogeneous, the divergence of this stress is trivially zero. The threshold activity number for the quiescent instability of bacterial suspension $\mathcal{A}^* = (Cn_0L^2U_b\tau) = (30\tau D_r/\mathcal{F}(r))(1 + 1/(6\tau D_r))/(1 - (15\mathcal{G}(r))/C\mathcal{F}(r))(D_rL/U_b)(1 + 1/(6\tau D_r))$ with $\mathcal{F}(r) \approx 1$ and $\mathcal{G}(r) \approx 0$ for a slender bacterium [S11]. The base state stress variation against shear rate for different $\mathcal{A}$ including the threshold activity number (bacterium with $\tau D_r = 1$, $\mathcal{A}^* \approx 35$) is shown in Fig. 2(a) in the main text.

## III. LINEAR STABILITY ANALYSIS

### A. Derivation of semi-analytical expression for the growth rate using a multiple scales analysis

In the limit $\epsilon \ll 1$, on account of the separation of time scales between the orientation and spatial degrees of freedom, one may use a multiple scales analysis to analyze the linear stability of the sheared homogeneous state. Accordingly, the time derivative is expanded as:

$$\frac{\partial}{\partial t} = \frac{\partial}{\partial t_1} + \epsilon^2 \frac{\partial}{\partial t_2}. \tag{S23}$$

Expanding the probability density as:

$$\Omega_1 = \Omega_{10} + \epsilon\Omega_{11} + \epsilon^2\Omega_{12} + \cdots \tag{S24}$$

and substituting this expansion in Eq. (S8), with the neglect of short time scale characterizing the orientation dynamics (as represented by $\partial/\partial t_1$), one obtains:

$$\mathcal{O}(1) : Pe\nabla_p.(\Omega_{10}\dot{\mathbf{p}}^{'}) + [\Omega_{10} - \int d\mathbf{p}^{'} \frac{1}{4\pi}\Omega_{10}(\mathbf{p}^{'})] - \tau D_r \nabla_p^2 \Omega_{10} = -Pe\dot{\gamma}_1 \nabla_p.(\Omega_0 \dot{\mathbf{p}}^{'}), \tag{S25}$$

$$\mathcal{O}(\epsilon) : Pe\nabla_p.(\Omega_{11}\dot{\mathbf{p}}^{'}) + [\Omega_{11} - \int d\mathbf{p}^{'} \frac{1}{4\pi}\Omega_{11}(\mathbf{p}^{'})] - \tau D_r \nabla_p^2 \Omega_{11} = -\mathbf{p}.\nabla_{\mathbf{x}}\Omega_{10}, \tag{S26}$$

$$\mathcal{O}(\epsilon^2) : Pe\nabla_p.(\Omega_{12}\dot{\mathbf{p}}^{'}) + [\Omega_{12} - \int d\mathbf{p}^{'} \frac{1}{4\pi}\Omega_{12}(\mathbf{p}^{'})] - \tau D_r \nabla_p^2 \Omega_{12} = -\frac{\partial \Omega_{10}}{\partial t_2} - \mathbf{p}.\nabla_{\mathbf{x}}\Omega_{11}. \tag{S27}$$

Equations S25-S27 are complemented by the following normalization conditions:

$$\int d\mathbf{p}\Omega_{10} = n_1(z, t_2), \tag{S28}$$

$$\int d\mathbf{p}\Omega_{11} = \int d\mathbf{p}\Omega_{12} = 0. \tag{S29}$$

On account of linearity, we postulate the following form for $\Omega_{10}$ to solve Eq. S25:

$$\Omega_{10} = \Omega_{10}^1 \dot{\gamma}_1(z, t_2) + \Omega_{10}^2 n_1(z, t_2), \tag{S30}$$

where $\Omega_{10}^1$ is the particular solution that integrates to zero over orientation space, while $\Omega_{10}^2$ is the homogeneous solution that confirms to the aforementioned normalization constraint. Through the active stress in the equations of motion, the perturbation in the probability density function ($\Omega_1$) drives the perturbation shear rate ($\dot{\gamma}_1$). In the following, we derive a reduced relation between them.

Substituting S30 in Eq. S25, S28, and equating the $\dot{\gamma}_1$ and $n_1$ terms, one obtains:

$$[\Omega_{10}^1 - \int d\mathbf{p}^{'} \frac{1}{4\pi}\Omega_{10}^1(\mathbf{p}^{'})] - \tau D_r \nabla_p^2 \Omega_{10}^1 + Pe\nabla_p.(\Omega_{10}^1 \dot{\mathbf{p}}^{'}) = -Pe\nabla_p.(\Omega_0 \dot{\mathbf{p}}^{'}), \tag{S31}$$

$$[\Omega_{10}^2 - \int d\mathbf{p}^{'} \frac{1}{4\pi}\Omega_{10}^2(\mathbf{p}^{'})] - \tau D_r \nabla_p^2 \Omega_{10}^2 + Pe\nabla_p.(\Omega_{10}^2 \dot{\mathbf{p}}^{'}) = 0, \tag{S32}$$

with the respective integral constraints being:

$$\int d\mathbf{p}\Omega_{10}^1 = 0, \tag{S33}$$

and

$$\int d\mathbf{p}\Omega_{10}^2 = 1. \tag{S34}$$

The unknown component probability densities $\Omega_{10}^1$ and $\Omega_{10}^2$ in Eq. S31-S34 will again be determined from an expansion in spherical harmonics. Thus writing:

$$\begin{aligned} \Omega_{10}^1 &= \sum_{l=0}^{\infty} \sum_{m=-l}^{m=l} c_{l,m} Y_l^m, \\ \Omega_{10}^2 &= \sum_{l=0}^{\infty} \sum_{m=-l}^{m=l} d_{l,m} Y_l^m, \end{aligned} \tag{S35}$$

the unknown coefficients $c_{l,m}$ and $d_{l,m}$ in the resulting equations can be obtained by employing the numerical scheme similar to the one mentioned in Supplementary Sec. I while evaluating $\Omega_0(\mathbf{p})$.

Substituting $\Omega_{10}$ from Eq. S30 in the right hand side of Eq. S26, we have

$$[\Omega_{11} - \int d\mathbf{p}' \frac{1}{4\pi}\Omega_{11}(\mathbf{p}')] - \tau D_r \nabla_p^2 \Omega_{11} + Pe \nabla_p.(\Omega_{11}\dot{\mathbf{p}}') = -\mathbf{p}.\nabla_x \Omega_{10}$$
$$= -\cos\theta \sum_{l'=0}^{\infty} \sum_{m'=-l'}^{l'} \left[ c_{l',m'} \frac{\partial \dot{\gamma}_1}{\partial z} + d_{l',m'} \frac{\partial n_1}{\partial z} \right] Y_{l'}^{m'}(\mathbf{p}). \tag{S36}$$

Again, on account of linearity, one may write:

$$\Omega_{11} = \Omega_{11}^1 \frac{\partial \dot{\gamma}_1}{\partial z} + \Omega_{11}^2 \frac{\partial n_1}{\partial z} \tag{S37}$$

and substituting in Eq. S29, S36, and equating the coefficients of $\frac{\partial \dot{\gamma}_1}{\partial z}$ and $\frac{\partial n_1}{\partial z}$, we get

$$[\Omega_{11}^1 - \int d\mathbf{p}' \frac{1}{4\pi}\Omega_{11}^1(\mathbf{p}')] - \tau D_r \nabla_p^2 \Omega_{11}^1 + Pe \nabla_p.(\Omega_{11}^1 \dot{\mathbf{p}}') = -\cos\theta \sum_{l'=0}^{\infty} \sum_{m'=-l'}^{l'} c_{l',m'} Y_{l'}^{m'}, \tag{S38}$$

$$[\Omega_{11}^2 - \int d\mathbf{p}' \frac{1}{4\pi}\Omega_{11}^2(\mathbf{p}')] - \tau D_r \nabla_p^2 \Omega_{11}^2 + Pe \nabla_p.(\Omega_{11}^2 \dot{\mathbf{p}}') = -\cos\theta \sum_{l'=0}^{\infty} \sum_{m'=-l'}^{l'} d_{l',m'} Y_{l'}^{m'}, \tag{S39}$$

with trivial normalization constraints given by:

$$\int \Omega_{11}^1 d\mathbf{p} = \int \Omega_{11}^2 d\mathbf{p} = 0. \tag{S40}$$

The probability densities $\Omega_{11}^1$, $\Omega_{11}^2$ can again be expanded as $\Omega_{11}^1 = \sum_{l=0}^{\infty} \sum_{m=-l}^{m=l} e_{l,m} Y_l^m$, $\Omega_{11}^2 = \sum_{l=0}^{\infty} \sum_{m=-l}^{m=l} f_{l,m} Y_l^m$. Substitution in Eq. S38-S40 allows one to solve for the unknown coefficients $e_{l,m}, f_{l,m}$ obtained by employing the numerical scheme as mentioned before.

Using Eq. S33, S34 and S37 in Eq. S27 and integrating over the orientation degrees of freedom, one obtains the following drift-diffusivity equation [S7, S9] at $\mathcal{O}(A)$:

$$\frac{\partial n_1}{\partial t_2} = \frac{\partial}{\partial z} \left( V_1(z).1 + D_0 \frac{\partial n_1}{\partial z} \right) \tag{S41}$$

in position space alone. Here $V_1 = -2\sqrt{\frac{\pi}{3}} e_{1,0} \frac{\partial \dot{\gamma}_1}{\partial z}$ is the destabilizing drift that multiplies the base-state number density (1 in non-dimensional terms) and $D_0 = -2\sqrt{\frac{\pi}{3}} f_{1,0}$ is the stabilizing diffusivity. Eq S41 is given as Eq 3 in the main text.

The variation in the perturbation shear rate is driven by the probability density variation, and hence the perturbation stress, through the equations of motion. Substituting the Eq. S5 and S6 in Eq. S4, the equilibrium equation at $\mathcal{O}(A)$:

$$Pe \frac{\partial^2 u_1(z, t_2)}{\partial z^2} = \mathcal{A} \frac{\partial}{\partial z} \int d\mathbf{p} \Omega_1(\mathbf{p}, z, t_2) p_1 p_3. \tag{S42}$$

Substituting $\Omega_1 = \Omega_{10} + \epsilon \Omega_{11} + \epsilon^2 \Omega_{12} + \cdots$, using Eq. S30 and S35 in the above equation and equating the leading order terms on both sides

$$Pe \frac{\partial^2 u_1(z, t_2)}{\partial z^2} = \mathcal{A} \frac{\partial}{\partial z} \int d\mathbf{p} \left[ \sum_{l=0}^{\infty} \sum_{m=-l}^{l} (\dot{\gamma}_1(z, t_2) c_{l,m} + n_1(z, t_2) d_{l,m}) Y_l^m(p) \right] \sqrt{\frac{2\pi}{15}} (Y_2^{-1}(p) - Y_2^1(p)).$$

$$\Rightarrow \frac{\partial \dot{\gamma}_1(z,t_2)}{\partial z}\left[Pe - \mathcal{A}\sqrt{\frac{2\pi}{15}}\left(c_{2,-1}-c_{2,1}\right)\right] = \mathcal{A}\sqrt{\frac{2\pi}{15}}\left(d_{2,-1}-d_{2,1}\right)\frac{\partial n_1(z,t_2)}{\partial z}. \tag{S43}$$

Using the normal mode forms $n_1(z,t_2) = \tilde{n}_1\cos(zk_z)\exp(\sigma t_2)$, $\dot{\gamma}_1(z,t_2) = \tilde{\dot{\gamma}}_1\cos(zk_z)\exp(\sigma t_2)$ in the above equation, we get

$$\tilde{\dot{\gamma}}_1 = \tilde{n}_1\frac{\sqrt{\frac{2\pi}{15}}\mathcal{A}(d_{2,-1}-d_{2,1})}{\left[Pe - \sqrt{\frac{2\pi}{15}}\mathcal{A}(c_{2,-1}-c_{2,1})\right]}. \tag{S44}$$

Substituting $\dot{\gamma}_1$ and $n_1$ in Eq. S41, using S44, one would get the growth rate expression as

$$\sigma = 2k_z^2\sqrt{\pi/3}\left(e_{1,0}\frac{\mathcal{A}\sqrt{\frac{2\pi}{15}}(d_{2,-1}-d_{2,1})}{\mu_0} - \frac{D_0}{2\sqrt{\frac{\pi}{3}}}\right), \tag{S45}$$

where $\mu_0 = Pe - \mathcal{A}\sqrt{\frac{2\pi}{15}}(c_{2,-1}-c_{2,1})$ is the viscosity of the homogeneously sheared state, which is analogous to the base-state stress obtained above, in its dependence on the coefficients of $\Omega_1$. The expression for growth rate, give in S45 appears as Eq. 4 in the main text.

### B. Numerical solution for the growth rate of Coupled Concentration-Orientation Dynamics

In this section we describe the numerical formulation for the full linear stability analysis without any assumption with regard to a time scales separation. As before, introducing a layering perturbation, and an amplitude $A \ll 1$, to the base-state simple shear, of the form:

$$u(z,t) = u_0(z) + Au_1(z,t) + \cdots, \tag{S46}$$

with the corresponding perturbations to the probability density and shear rate being:

$$\Omega = \Omega_0(\mathbf{p}) + A\Omega_1(\mathbf{p},z,t) + \cdots, \tag{S47}$$

$$\dot{\gamma}(z,t) = \frac{\partial u}{\partial z} = \dot{\gamma}_0 + A\dot{\gamma}_1(z,t) + \cdots, \tag{S48}$$

substituting Eq. S47 and S48 in S1 and collecting terms at successive orders, one obtains:

$$\mathcal{O}(1): \dot{\gamma}_0\nabla_p(\dot{\mathbf{p}}'\Omega_0) - D_r\nabla_p^2\Omega_0 + \frac{1}{\tau}[\Omega_0 - \int d\mathbf{p}'\frac{1}{4\pi}\Omega_0(\mathbf{p}')] = 0, \tag{S49}$$

$$\mathcal{O}(A): \frac{\partial\Omega_1}{\partial t} + U_b\mathbf{p}.\nabla_{\mathbf{x}}\Omega_1 - D_r\nabla_p^2\Omega_1 + \dot{\gamma}_0\nabla_p(\dot{\mathbf{p}}'\Omega_1) + \dot{\gamma}_1\nabla_p(\dot{\mathbf{p}}'\Omega_0) + \frac{1}{\tau}[\Omega_1 - \int d\mathbf{p}'\frac{1}{4\pi}\Omega_1(\mathbf{p}')] = 0. \tag{S50}$$

Using $\tau$, $U_b\tau$ (as opposed to $H$ in the multiple scales analysis earlier), $U_b$ are the scales for time, length, velocity, Eq. S49 and S50 in dimensionless form are given by:

$$\mathcal{O}(1): Pe\nabla_p(\dot{\mathbf{p}}'\Omega_0) - \tau D_r\nabla_p^2\Omega_0 + [\Omega_0 - \int d\mathbf{p}'\frac{1}{4\pi}\Omega_0(\mathbf{p}')] = 0, \tag{S51}$$

$$\mathcal{O}(A): \frac{\partial\Omega_1}{\partial t} + \mathbf{p}.\nabla_{\mathbf{x}}\Omega_1 - \tau D_r\nabla_p^2\Omega_1 + Pe\nabla_p(\dot{\mathbf{p}}'\Omega_1) + \dot{\gamma}_1\nabla_p(\dot{\mathbf{p}}'\Omega_0) + [\Omega_1 - \int d\mathbf{p}'\frac{1}{4\pi}\Omega_1(\mathbf{p}')] = 0, \tag{S52}$$

where $Pe = \dot{\gamma}_0\tau$.

Assuming the usual normal mode form:

$$\Omega_1(z,\mathbf{p},t) = \tilde{\Omega}_1(k_z,\mathbf{p})\exp(izk_z + \sigma t) \tag{S53}$$

and

$$u_1(z,t) = \tilde{u}_1(k_z)\exp(izk_z + \sigma t) \tag{S54}$$

and substituting in Eq. S52, one obtains:

$$\tilde{\Omega}_1\sigma + (ik_z\cos\theta)\tilde{\Omega}_1 + Pe\nabla_p.(\dot{\mathbf{p}}^{'}\tilde{\Omega}_1) + ik_z\tilde{u}_1\nabla_p.(\dot{\mathbf{p}}^{'}\tilde{\Omega}_0) - \tau D_r\nabla_p^2\tilde{\Omega}_1 + [\tilde{\Omega}_1 - \int d\mathbf{p}^{'}\frac{1}{4\pi}\tilde{\Omega}_1(\mathbf{p}^{'})] = 0. \tag{S55}$$

Substituting Eq. S46, S47 in Eq. S2, then the momentum equation, at $\mathcal{O}(A)$, takes the form:

$$\frac{\partial^2 u_1}{\partial z^2} = \mathcal{A}\frac{\partial}{\partial z}\int d\mathbf{p}\Omega_1(z,\mathbf{p})p_1p_3. \tag{S56}$$

Using, Eq.S53 and S54 in the above equation, one has the following relation coupling the perturbation shear to the probability density:

$$\tilde{u}_1 = -\frac{i\mathcal{A}}{k_z}\int d\mathbf{p}\tilde{\Omega}_1(k_z,\mathbf{p})p_1p_3. \tag{S57}$$

Using $\tilde{u}_1$ from Eq. S57 in $\tilde{u}_1$ in Eq. S55, one obtains:

$$Pe\nabla_p.(\dot{\mathbf{p}}^{'}\tilde{\Omega}_1)+(ik_z\cos\theta)\tilde{\Omega}_1+\mathcal{A}\left(\int d\mathbf{p}\tilde{\Omega}_1(k_z,\mathbf{p})p_1p_3\right)\nabla_p.(\dot{\mathbf{p}}^{'}\Omega_0)-\tau D_r\nabla_p^2\tilde{\Omega}_1+[\tilde{\Omega}_1-\int d\mathbf{p}^{'}\frac{1}{4\pi}\tilde{\Omega}_1(\mathbf{p}^{'})] = -\tilde{\Omega}_1\sigma. \tag{S58}$$

The unknown $\Omega_0$ in the above equation obtained numerically, as already explained in terms of a spherical harmonic series (see Supplementary Sec. I). Substituting the known from for $\Omega_0$, expanding

$$\tilde{\Omega}_1 = \sum_{l=0}^{N}\sum_{m=-l}^{l} b_{l,m}Y_l^m(\mathbf{p}) \tag{S59}$$

in terms of spherical harmonics, and following the numerical procedure as mentioned in Supplementary Sec. I, we solve the resulting eigenvalue problem. The variation in the leading growth rate value of coupled concentration-orientation dynamics (real($\sigma$)) and the the growth rate value of concentration dynamics against $Pe$ has been compared in Fig. 3 in the main text.

## IV. NUMBER DENSITY PERTURBATIONS

The normalization condition of the bacterial probability density (Eq. S17) gives

$$\int d\mathbf{p}\Omega_1 = n_1. \tag{S60}$$

Substituting $\Omega_1$ from Eq. S53 and using $n_1 = \tilde{n}_1\exp(izk_z + \sigma t)$ in the above equation, one obtains:

$$\int d\mathbf{p}\tilde{\Omega}_1 = \tilde{n}_1. \tag{S61}$$

Now substituting $\tilde{\Omega}_1$ expansion from Eq. S59 in the above equation and after simplification, we obtain the number density perturbation amplitude $\tilde{n}_1 = \sqrt{4\pi}b_{0,0}$. The leading growth rate value (real($\sigma$)), and the corresponding number density perturbation against wave number for different $Pe$ have been plotted in Fig. 4.

## V. NON-LINEAR SIMULATIONS

For the non-linear simulations, the bacterial orientations are assumed to be confined to the shear-gradient plane, so in contrast to that shown in Fig. S1, $\mathbf{p}$ in the simulations is taken as $\cos\theta 1_x + \sin\theta 1_z$. The Stokes equations are used to express the shear rate variation along the gradient direction in terms of $\Omega$, so that the kinetic equation takes the

form of a non-linear integro-differential equation for $\Omega$. Then the orientation and spatial dependence of the unknown variable, $\Omega$, is expanded in a Fourier series as follows:

$$\Omega = \sum_{m=-N_p}^{N_p} \sum_{k=-N_k}^{N_k} a_m^k e^{(ikz+im\theta)} \tag{S62}$$

A standard Galerkin projection gives a set of coupled ODEs for $a_m^k$ which are integrated in time using a second order Runge-Kutta scheme [S3, S4]. Convergence is checked with respect to both $N_p$ and $N_k$ and it is found that 17 orientation harmonics and 301 spatial harmonics are sufficient for convergence for all the results presented in the paper.

The steady state can comprise of multiple bands depending on the particular initial condition, as is known from earlier work on passive complex fluids [S6]. Thus a suitable initial condition is chosen for which the minimum number of bands are present in the steady state.


[S1] Arfken, G. B., and Weber, H. J. Mathematical methods for physicists, 1999.

[S2] Batchelor, G. The stress system in a suspension of force-free particles. *Journal of fluid mechanics 41*, 3 (1970), 545–570.

[S3] Boyd, J. P. *Chebyshev and Fourier spectral methods.* Courier Corporation, 2001.

[S4] Canuto, C., Hussaini, M. Y., Quarteroni, A., Thomas Jr, A., et al. *Spectral methods in fluid dynamics.* Springer Science & Business Media, 2012.

[S5] Doi, M., and Edwards, S. F. Dynamics of rod-like macromolecules in concentrated solution. part 2. *Journal of the Chemical Society, Faraday Transactions 2: Molecular and Chemical Physics 74* (1978), 918–932.

[S6] Fielding, S. M., and Olmsted, P. D. Flow phase diagrams for concentration-coupled shear banding. *The European Physical Journal E 11*, 1 (2003), 65–83.

[S7] Kasyap, T., and Koch, D. L. Chemotaxis driven instability of a confined bacterial suspension. *Physical review letters 108*, 3 (2012), 038101.

[S8] Messiah, A. *Quantum Mechanics [Vol 2].* 1962.

[S9] Nitsche, L. C., and Hinch, E. Shear-induced lateral migration of brownian rigid rods in parabolic channel flow. *Journal of Fluid Mechanics 332* (1997), 1–21.

[S10] Saintillan, D., and Shelley, M. J. Instabilities and pattern formation in active particle suspensions: kinetic theory and continuum simulations. *Phys. Rev. Lett. 100*, 17 (2008), 178103.

[S11] Subramanian, G., and Koch, D. L. Critical bacterial concentration for the onset of collective swimming. *Journal of Fluid Mechanics 632* (2009), 359–400.
